# Supplementary material for: Redistribute Ensemble Training for Mitigating Memorization in Diffusion Models
Source: arXiv:2502.09434 source file (2025-02-13)
Supplement: Supplementary file 1 [file supp_1.tex]

% \appendices
\appendix
\section*{Loss Analysis on CIFAR-100, AFHQ-DOG, and LAION-10k }
We present the results of loss analysis for CIFAR-100, AFHQ-DOG, and LAION-10k in \cref{fig:cifar100_loss}, \cref{fig:afhq_loss}, and \cref{fig:laion_loss}. 
The results obtained on CIFAR-100 and LAION-10k show similarities to those on CIFAR-10. 
However, on AFHQ-DOG, due to its fewer images, the model exhibits a memorization phenomenon across the entire dataset, resulting in less noticeable differences.
% \vspace{-0.7cm}
\begin{figure}[t]
  \centering
  \setlength{\abovecaptionskip}{-4pt} % 设置标题上方的间距为 -5pt
  \setlength{\belowcaptionskip}{-10pt} % 设置标题下方的间距为 -5pt
  \includegraphics[height=6.5cm]{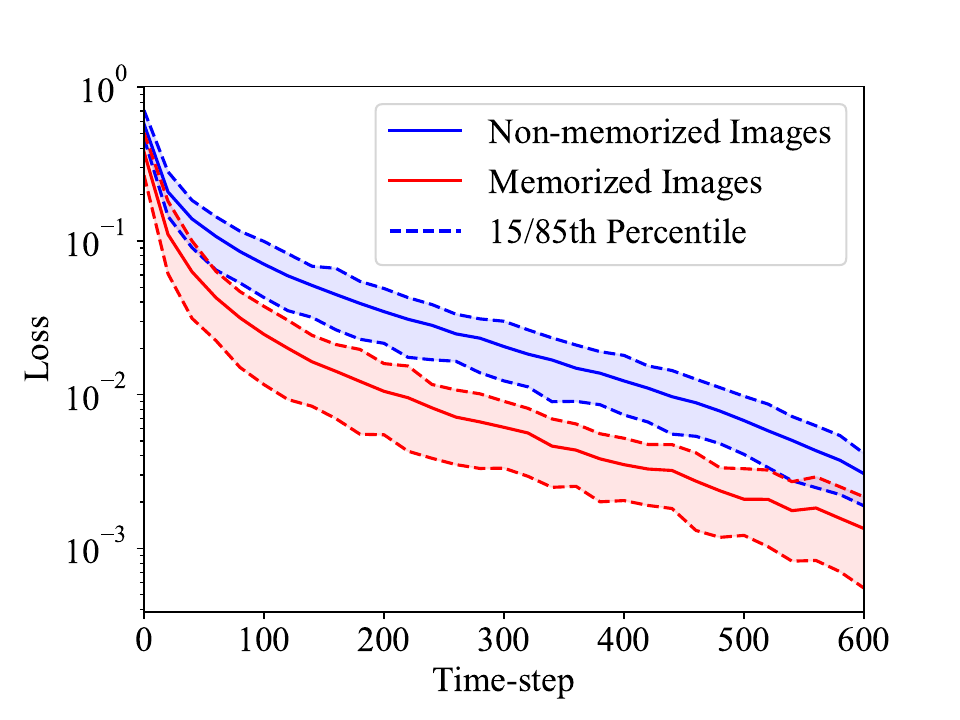}
  \caption{
  Comparison of the losses between memorized and non-memorized images on CIFAR-100. 
  }
  \label{fig:cifar100_loss}
\end{figure}
% \clearpage
% \vspace*{0pt}
\begin{figure}[t]
  \centering
  \setlength{\abovecaptionskip}{-4pt} % 设置标题上方的间距为 -5pt
  \setlength{\belowcaptionskip}{-10pt} % 设置标题下方的间距为 -5pt
  \includegraphics[height=6.5cm]{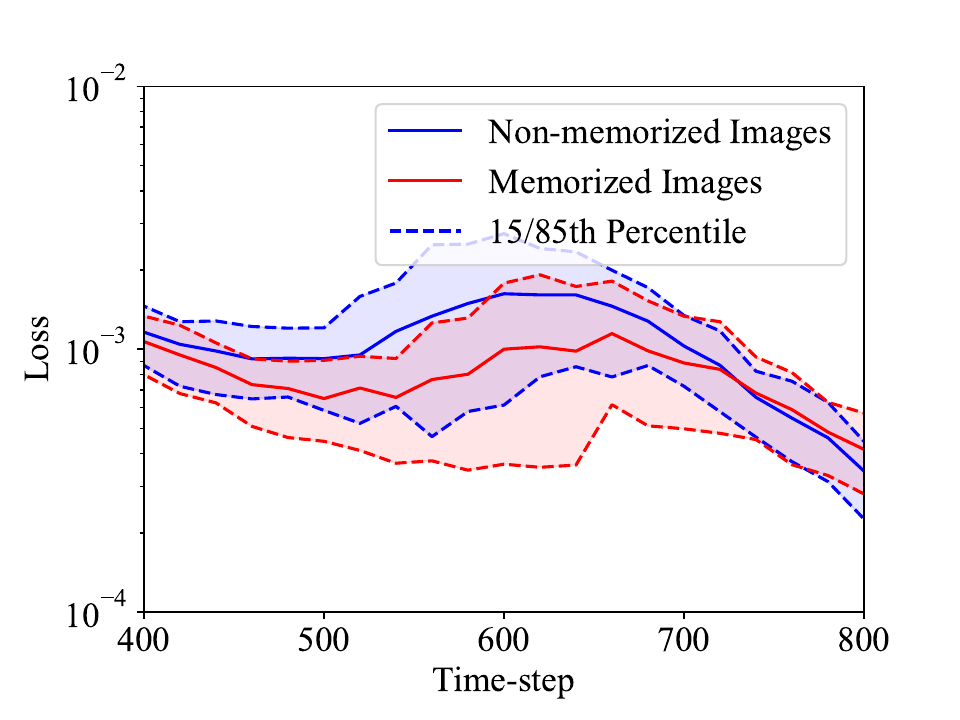}
  \caption{
  Comparison of the losses between memorized and non-memorized images on AFHQ-DOG.
  }
  \label{fig:afhq_loss}
\end{figure}

\vspace*{0pt}
\begin{figure}[t]
  \centering
  \setlength{\abovecaptionskip}{-4pt} % 设置标题上方的间距为 -5pt
  \setlength{\belowcaptionskip}{-5pt} % 设置标题下方的间距为 -5pt
  \includegraphics[height=6.5cm]{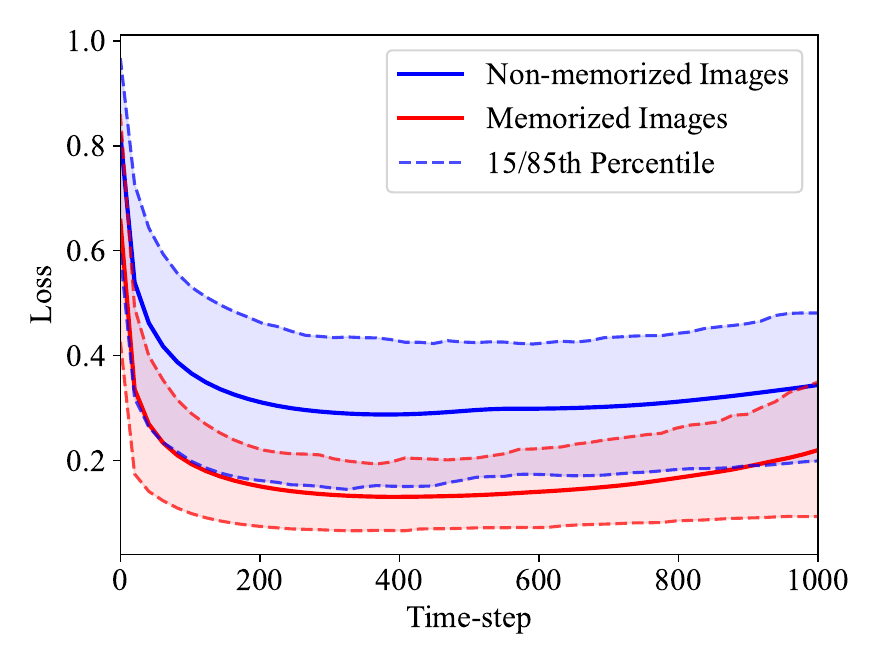}
  \caption{
  Comparison of the losses between memorized and non-memorized images on LAION-10k. 
  }
  \label{fig:laion_loss}
\end{figure}

\section*{Experiments of DP-SGD with varying noise multipliers}
We conduct a series of experiments with DP-SGD (Differentially-Private Stochastic Gradient Descent)~\cite{abadi2016deep} changing the noise multipliers $\tau$ to 0.0002, 0.0005, and 0.0008 to compare our method with different noise levels in DP. Results are shown in ~\cref{tab:dp_parameters}.  When the noise multiplier is set to 0.0005, DP-SGD achieves the best scores in terms of MQ and FID. However, all DP-SGD results improve the FID score compared with the baseline model. When $\tau$=0.0005, DP-SGD slightly reduces the memorization (101 v.s. 111), but it is still far from comparable to the memorization reduction capability of our method.
%our method still surpasses it, demonstrating lower memory usage and superior image quality.
% Table generated by Excel2LaTeX from sheet 'Sheet1'
% \vspace{-0.5cm}
\begin{table}[t]
  \centering
  \caption{Performance of DP-SGD across multiple experiments with varying noise multiplier $\tau$.}
  {\fontsize{6.5}{8}\selectfont %
    \begin{tabular}{c|ccc|c}
    \specialrule{\heavyrulewidth}{0pt}{0pt} % 加粗的水平线，位于表格底部
    \hline
    \multirow{2}[4]{*}{Method} & \multicolumn{4}{c}{CIFAR-10} \bigstrut\\
\cline{2-5}         & MQ$_{0.4}$ & MQ$_{0.5}$ & MQ$_{0.6}$$\downarrow$ & FID$\downarrow$  \bigstrut\\
    \hline
    \hline
    Default (DDPM)~\cite{ho2020denoising} & 111   & 465   & 2030  & 8.81 \bigstrut[t]\\
    DP-SGD~\cite{abadi2016deep} $\tau$=0.0002 & 148   & 728   & 3200  & 12.55 \\
    DP-SGD~\cite{abadi2016deep} $\tau$=0.0005 & 101   & 380   & 1716  & 10.02 \\
    DP-SGD~\cite{abadi2016deep} $\tau$=0.0008 & 124   & 549   & 2498  & 13.82 \bigstrut[b]\\
    \hline
    Ours & \textbf{10} & \textbf{73} & \textbf{623} & \textbf{8.33} \bigstrut\\
    \hline
     \specialrule{\heavyrulewidth}{0pt}{0pt} % 加粗的水平线，位于表格底部
    \end{tabular}%
    }
  \label{tab:dp_parameters}%
\end{table}%

\section*{More Ablation Study}
\crnote{We randomly split the data evenly on AFHQ-DOG and LAION-10k, where no class label is available on these datasets.
Experiments demonstrate the effectiveness of our method in this setting.
Additionally, we conduct ablation experiments on CIFAR-10 by randomly splitting the data evenly (without using class labels). Results are shown in ~\cref{tab:nonclass}.
% We believed that a uniformly distributed class was better for the model’s performance.
We find randomly splitting (without class labels) slightly affects the generation quality. }
\begin{table}[t]
  \centering
  \caption{Ablation experiments of randomly splitting the data evenly.}
  % \vspace{-1.1em}
  % \setlength{\abovecaptionskip}{-40pt}
    {\fontsize{6.5}{8}\selectfont %
    \begin{tabular}{P{3.0cm}|P{1.0cm}P{1.0cm}P{1.0cm}|P{0.8cm}}
     \specialrule{\heavyrulewidth}{0pt}{0pt} % 加粗的水平线，位于表格底部
    \hline
    \multirow{2}[4]{*}{Method} & \multicolumn{4}{c}{CIFAR-10}  \bigstrut\\
\cline{2-5}        & MQ$_{0.4}$  & MQ$_{0.5}$ & MQ$_{0.6}$$\downarrow$ & FID$\downarrow$   \bigstrut\\
    \hline
    \hline
    Default (DDPM)~\cite{ho2020denoising} & 111 & 465   & 2030  & 8.81 \bigstrut\\
     
    IET-AGC (w/o class label) & \textbf{10} & \textbf{91} & \textbf{769} & 9.12  \bigstrut\\
    IET-AGC (w/ class label)& 14   & 117  & 839 & \textbf{8.34}  \bigstrut\\
    \hline
    \specialrule{\heavyrulewidth}{0pt}{0pt} % 加粗的水平线，位于表格底部
    \end{tabular}%
    
    }
    \label{tab:nonclass}%
    % \vspace{-1.6em}
\end{table}%
\section*{Implementational Details}
\crnote{
When conducting experiments on training Diffusion models from scratch using CIFAR-10 and CIFAR-100, we set the batch size to 128 and train for 400k and 580k iterations, respectively. 
On AFHQ-DOG, the batch size is set to 60, and we train for 180k iterations. 
In the IET framework, CIFAR-10 and CIFAR-100 are divided into ten shards, each containing the same number of classes and instances.
AFHQ-DOG is divided into five shards based on the number of instances, as it lacks class information. 
On the CIFAR-10 and CIFAR-100 datasets, we set the threshold $\lambda$ to $0.5$, indicating that data with loss less than half of the average loss is skipped. 
For the AFHQ-DOG dataset, due to its smaller size and pronounced memory phenomena, we adjust the threshold $\lambda$ to $0.714$.
To demonstrate the effectiveness of our method in text-conditioned Diffusion models, we fine-tune Stable Diffusion on LAION-10k. 
The IET framework divides the LAION-10k dataset into 4 shards, with the threshold $\lambda$ set to 0.8. 
We set the batch size to 8 and fine-tune Stable Diffusion for 200k iterations.
On all datasets, the smoothing factor $\gamma$ for the memory bank is set to 0.8. 
}
\section*{\gxlnote{The IID and non-IID Setting in IET framework}}
In addition, in our approach, the dataset is evenly distributed, meaning each data shard is set in an IID (independently and identically distributed) manner. To validate the reasonableness of this dataset configuration, we also establish an experiment where each data shard is set up in a non-independent and identically distributed (non-IID) manner on CIFAR-10. Similar to Hsu \MakeLowercase{\textit{et al.}}~\cite{hsu2019measuring}, we employ the Dirichlet distribution to generate data, thereby establishing such a setting.
% Table generated by Excel2LaTeX from sheet 'Sheet1'
\begin{table}[t]
  \centering
  \caption{The results under the IID and non-IID setting in the IET framework.}
    \begin{tabular}{c|ccc|c}
    \specialrule{\heavyrulewidth}{0pt}{0pt} % 加粗的水平线，位于表格底部
    \hline
    \multirow{2}[4]{*}{Method} & \multicolumn{4}{c}{CIFAR-10} \bigstrut\\
\cline{2-5}          & MQ$_{0.4}$ & MQ$_{0.5}$ & MQ$_{0.6}$$\downarrow$  & FID↓ \bigstrut\\
    \hline
    \hline
    Default (DDPM)~\cite{ho2020denoising} & 111   & 465   & 2030  & 8.81 \bigstrut[t]\\
    IET$_\mathrm{non-IID}$ & \textbf{69} & \textbf{315} & \textbf{1439} & 12.5 \\
    IET$_\mathrm{IID}$ & 89    & 382   & 1783  & \textbf{7.61} \bigstrut[b]\\
    \hline
    \specialrule{\heavyrulewidth}{0pt}{0pt} % 加粗的水平线，位于表格底部
    \end{tabular}%
  \label{tab:ablation_IID}%
  \vspace{-8pt}
\end{table}%

Results in ~\cref{tab:ablation_IID} show that when the data shards are set in non-IID, Iterative Ensemble Training (IET) successfully reduces the memorization.
However, the non-IID splitting reduces the quality of performance since the divergent optimization of different models and aggregating these models affects the performance. 
Differently, when the data shards are set in IID,  IET$_\mathrm{IID}$ can reduce both the memorization and FID score. 
Thus in this paper, we choose to use the IID splitting strategy.

\section*{Algorithm}
A pseudo-code implementation is provided in ~\cref{algorithm}.
\vspace{-10pt}
\begin{algorithm}[htp]
\caption{The Proposed Framework}
\SetAlgoLined
\LinesNotNumbered
\KwIn{Dataset $D$, the number of dataset $N$, training rounds $M$, training epochs per interaction period $E$, number of shards $K$, initial model $\theta^0$, skipping threshold $\lambda$, smoothing factor $\eta$, memory bank $l$,  augmentation Range $R$,  skip time $s$ }
\KwOut{Diffusion model $\theta^M$}
Divide dataset $D$ into an equal number of shards $D_i$, $i\in [1,...,K]$\;
Initialize memory bank $l$ with all elements as $0$\;
Initialize skip time $s_i^j$ with all samples as $0$, $j\in [1,...,\frac{N}{K}]$, $i\in [1,...,K]$;

\For{$m=1$ \KwTo $M$}{
    \For{$i=1$ \KwTo $K$}{
        Initialize model $\theta_{i}^m \leftarrow \theta^{m-1}$\;
        \For{$e=1$ \KwTo $E$}{            
            $x \in D_i \quad \text{and} \quad \text{is} \quad  j\text{th} \quad \text{sample}$
            
            $\epsilon  \sim \mathit{N} (0, I) $ , $t$ $\sim$ Uniform $({1, ..., T})$\;       
            $Loss = \mathcal{L} (x, t, \epsilon; \theta_{i}^m)$ \\
% \tcp{Threshold-Aware Control}\\
            \If{$\frac{Loss}{l_t} < \lambda$}
            {
                $Loss \leftarrow 0$;
                $s_i^j=s_i^j +1$
            }
            \If{$\lambda<\frac{Loss}{l_t} < R\lambda$}
            {
                $Loss \leftarrow \mathcal{L}(\mathbf{Aug}(x, e^{-5\parallel \frac{ r - \lambda}{\lambda}\parallel}))$;
            }
            $l_{t} \leftarrow \eta \cdot l_t + (1 - \eta) \cdot \mathcal{L} (x, t, \epsilon; \theta_{i}^m)$ \\
             Then update $\theta_{i}^m$ by $Loss$
             % \leftarrow \theta_{i}^m - \eta \nabla Loss$
        }
    }
    \tcp{Model Aggregation}
    \If{$m \mod 2 == 0$}
    {
       $\theta^m\leftarrow \frac{1}{K}\sum_{i=1}^{K}\theta_{i}^m$
    }
    \tcp{Memory Samples Redistribute}
    \Else
    {
        \For{$i=1$ \KwTo $K$}{
                $Top_P \gets$ $Top_P(s_i^1, s_i^2, \dots, s_i^\frac{N}{K})$\;
                $D_i^{\text{easy}} \gets \emptyset$\;
        
        \For{$j = 1$ \KwTo $\frac{N}{K}$}{
            \If{$s_i^j \geq Top_P$}{
                $D_i^{\text{easy}} \cup \{x_j\} \rightarrow D_i^{\text{easy}}$ \;
            }
            $s_i^j \gets 0$
        }
         $D_{i + 1} \cup D_i^{\text{easy}}  \rightarrow D_{i + 1}$
        }
    }   
}
\label{algorithm}
\end{algorithm}
