# Supplementary material for: Redistribute Ensemble Training for Mitigating Memorization in Diffusion Models
Source: arXiv:2502.09434 source file (2025-02-13)
Supplement: Supplementary file 2 [file supp_2.tex]

\appendix
% \section{Appendix}
\setcounter{table}{0}
% \includesvg[inkscapelatex=false,width=1.3\linewidth]{other_objects2.svg}
In the supplementary material, Sec.~\ref{sec:generated_results} showcases an array of TV2I generation results along with comprehensive analyses. 
Furthermore, we conduct extensive qualitative and quantitative image comparisons with baseline methods, and detailed results of human evaluations are elaborated on. 
% in Sec.~\ref{sec:image_comparison_with_baselines}.  
Our analysis of different hyper-parameters of the number of cycles and positions of the start and end points can be found in Sec.~\ref{appen:hyperparameters}.
Our thorough ablation study shows the effectiveness of dynamic attention modulation and prompt intensification of the three settings (Sec.~\ref{ablation_study}).
Moreover, we illuminate the varying sensitivity to text conditions during the denoising process (Sec.~\ref{sec:text-sensitivity}) and elucidate the semantic formation process of diffusion generation (Sec.~\ref{sec:diff-size_semantic_formation}).

\section*{TV2I Generation Results Comparison and Analysis}\label{sec:generated_results}
\subsection{More Comparisons with Baselines}\label{sec:image_comparison_with_baselines}
\begin{table*}[!hb]
  \caption{Quantitative results of objective metrics on the CelebA-TV2I test set and human evaluations under the NORMAL setting.}
  \centering
  \setlength{\aboverulesep}{0pt}
  \setlength{\belowrulesep}{0pt}
  \scalebox{1}{
  \begin{tabular}{l|cc|cc}
    \bottomrule    
    & \multicolumn{2}{c|}{Objective Metrics} & \multicolumn{2}{c}{Human Evaluations} \\ \hline
    Methodology  & ID-Distance $\downarrow$ & Face Detection Rate $\uparrow$ & Condition Consistency $\uparrow$ & General Fidelity $\uparrow$ \\ \hline 
    TI               & 1.182 & 45.00\% & 2.83\% & 9.63\% \\
    DreamBooth       & 1.335 & 40.50\% & \underline{18.77\%} & \underline{21.98\%} \\
    ControlNet       & 1.011 & \underline{99.00\%} & 9.25\% & 2.72\% \\
    SD inpainting    & \textbf{0.389} & \textbf{100.00\%} & 9.25\% & 0.49\% \\
    SOW (ours)       & \underline{0.600} & \textbf{100.00\%} & \textbf{65.19\%} & \textbf{51.87\%} \\
    \bottomrule
  \end{tabular}}
  \label{tab:basic-metrics-normal}
\end{table*}
\begin{table*}[!hb]
  \caption{Quantitative results of objective metrics on the CelebA-TV2I test set and human evaluations under the STYLE TRANSFER setting.}
  \centering
  \setlength{\aboverulesep}{0pt}
  \setlength{\belowrulesep}{0pt}
  \scalebox{1}{
  \begin{tabular}{l|cc|cc}
    \bottomrule    
    & \multicolumn{2}{c|}{Objective Metrics} & \multicolumn{2}{c}{Human Evaluations} \\ \hline 
    Methodology  & ID-Distance $\downarrow$ & Face Detection Rate $\uparrow$ & Condition Consistency $\uparrow$ & General Fidelity $\uparrow$ \\ \hline 
    TI               & 1.212 & 41.50\% & 3.92\% & 13.42\% \\
    DreamBooth       & 1.323 & 41.50\% & \underline{22.79\%} & \underline{35.70\%} \\
    ControlNet       & 1.193 & \underline{92.50\%} & 13.48\% & 5.57\% \\
    SD inpainting    & \textbf{0.400} & \textbf{100.00\%} & 9.07\% & 1.52\% \\
    SOW (ours)       & \underline{1.027} & \textbf{100.00\%} & \textbf{50.74\%} & \textbf{43.80\%} \\
    \bottomrule
  \end{tabular}}
  \label{tab:basic-metrics-style}
\end{table*}

\begin{table*}[!hb]
  \caption{Quantitative results of objective metrics on the CelebA-TV2I test set and human evaluations under the ATTRIBUTE EDITING setting.}
  \centering
  \setlength{\aboverulesep}{0pt}
  \setlength{\belowrulesep}{0pt}
  \scalebox{1}{
  \begin{tabular}{l|cc|cc}
    \bottomrule    
    & \multicolumn{2}{c|}{Objective Metrics} & \multicolumn{2}{c}{Human Evaluations} \\ \hline 
    Methodology  & ID-Distance $\downarrow$ & Face Detection Rate $\uparrow$ & Condition Consistency $\uparrow$ & General Fidelity $\uparrow$ \\ \hline 
    TI               & 1.212 & 42.00\% & 3.55\% & 8.17\% \\
    DreamBooth       & 1.320 & 34.00\% & \underline{33.57\%} & \underline{39.11\%} \\
    ControlNet       & 1.073 & \underline{97.00\%} & 5.20\% & 1.49\% \\
    SD inpainting    & \textbf{0.401} & \textbf{100.00\%} & 3.31\% & 1.73\% \\
    SOW (ours)       & \underline{0.686} & \textbf{100.00\%} & \textbf{54.37\%} & \textbf{49.50\%} \\
    \bottomrule
  \end{tabular}}
  \label{tab:basic-metrics-editing}
\end{table*}

In Fig.~\ref{compare}, we include a more intuitive comparison with baseline results.
We compare current methods that incorporates visual conditions into pre-trained T2I models: DreamBooth~\cite{ruiz2022dreambooth}, TI~\cite{gal2022ti}, ControlNet~\cite{controlnet}, and SD inpainting~\cite{rombach2022ldm}. As shown in Tab.~\ref{tab:basic-metrics-normal}, Tab.~\ref{tab:basic-metrics-style}, and Tab.~\ref{tab:basic-metrics-editing}, our method works well and outperforms most baselines in most evaluation metrics across the three settings.

We conduct a human evaluation based on two criteria: 1) {Condition Consistency}: whether the generated image well matches both the visual and textual conditions; 2) {General Fidelity}: whether the chosen image looks more like a real image in terms of image richness, face naturalness, and overall image fidelity.  It is worth noting that we inform the participants of the application setting: input the face text condition pairs and then get an output image, and ask them to choose a favorite result if they were the users under the two basic criteria. The voting rate for our results greatly surpasses the other baselines in both criteria across all three settings, as shown in Tab.~\ref{tab:basic-metrics-normal}, Tab.~\ref{tab:basic-metrics-style}, and Tab.~\ref{tab:basic-metrics-editing}, and this demonstrates the general quality when applied to TV2I generation. 
% The participants recruited are all undergraduate or graduate students, all over 18 years old, ranging from 18-26 years old. Therefore, there are no ethical concerns for young participants (under 18 years old). Before taking the questionnaire, all participants are informed about the research's purpose, the compensation, and the user study content. All participants consent to participate. We do not provide compensation to volunteers. 
% In addition, all elements of the questionnaire are free from potential psychological or moral hazards. 

% We show interface examples of questionnaire systems received by participants regarding these two criteria in Fig.~\ref{fig:human_evaluation1} and Fig.~\ref{fig:human_evaluation2}.
 \begin{table}[!h]
    \centering
    \caption{Comparison of different hyper-parameters of the cycle number and the cycle position on the CelebA-TV2I validation set.}
    \label{Tab:different_hyper-parameters.}
    \vspace{0mm} % Adjust vertical space above the table
    \setlength{\aboverulesep}{0pt} % No space above the horizontal rules
    \setlength{\belowrulesep}{0pt} % No space below the horizontal rules
    \resizebox{0.5\textwidth}{!}{
    \begin{tabular}{cc|ccc}
    \toprule
    Cycle & Position & ID-Distance $\downarrow$ & Face Detection Rate $\uparrow$ & Time Cost $\downarrow$ \\ \hline \hline
    10 & 700 $\rightarrow$ 500 & 0.8068 & 100.00\% & 4.67 \\
    \hdashline
    10 & 900 $\rightarrow$ 700 & 1.0520 & 96.67\% & 4.93 \\
    10 & 800 $\rightarrow$ 400 & 0.7194 & 98.33\% & 9.59\\
    10 & 500 $\rightarrow$ 300 & 0.6606 & 98.33\% & 5.08\\
    \hdashline
    5 & 700 $\rightarrow$ 500 & 0.6726 & 100.00\% & 2.45 \\
    20 & 700 $\rightarrow$ 500 & 0.6714 & 100.00\% & 9.65 \\
    \bottomrule
    \end{tabular}
    }
\end{table}
\subsection{More Analysis of Different Hyper-parameters}
\label{appen:hyperparameters}
We conduct an analysis of different hyper-parameters of SOW, including the number of cycles, or positions of the start and end points in Tab.~\ref{Tab:different_hyper-parameters.}.
Here we use three quantitative metrics to analyze different models. 
% \textit{CLIP-T} is the CLIP-text cosine-similarity, which is the similarity of generated image and text condition calculated by the prestrained CLIP (ViT-B/32) model. 
% We also perform human evaluations on those ablation models with 10 volunteers to better evaluate the visual quality of the generated samples. (Each volunteer carefully goes through 216 images generated by the six model variants and rates the best model variant as 5 and the worst as 0, similar to the Mean of Score test in previous works~\cite{zhu2022quantized}. Here we report the averaged ratings for each model.) 
% We also include the time cost per image generation. 
Since different starting and ending points would involve different inversion steps, the time cost is slightly different according to the diffusion inversion cost. 
The results show that the model's performance is sensitive to the starting and ending points, which confirms our motivation to repeatedly go through the semantic formation stage to have a controllable and directional generation.
As we can see, a cycle number of 10 is sufficient and achieves a good balance between performance and speed for the inner diffusion process.

\subsection{More Ablation Study results}
\label{ablation_study}

% \begin{table}[!t]
%     \centering
%     \caption{Comparison of different hyper-parameters of the cycle number and the cycle position on the validation set.}
%     \label{Tab:different_hyper-parameters.}
%     \vspace{0mm} % Adjust vertical space above the table
%     \centering
%     \setlength{\aboverulesep}{0pt} % No space above the horizontal rules
%     \setlength{\belowrulesep}{0pt} % No space below the horizontal rules
%     \resizebox{0.5\textwidth}{!}{
%     \begin{tabular}{cc|ccccc}
%     \toprule
%     Cycle &Position &Clip-T $\uparrow$&Clip-I $\uparrow$& ID-Distance$\downarrow$&Face Dection Rate$\uparrow$&Time Cost$\downarrow$ \\ \hline \hline
%     % \midrule
%     10 & 700 $\rightarrow$ 500 & 0.2804&0.6132&0.8068 & 100.00\%  & 4.67 \\
%     \hdashline
%     10 & 900 $\rightarrow$ 700 & 0.2926 &0.5297&1.0520  & 96.67\% &4.93 \\
%     10 & 800 $\rightarrow$ 400 & 0.2898 &0.6003&0.7194  & 98.33\% &9.59\\
%     10 & 500 $\rightarrow$ 300 & 0.2629 &0.6664&0.6606&98.33\% & 5.08\\
%     \hdashline
%     5 & 700 $\rightarrow$ 500 & 0.2537 & 0.6772 &0.6726&100.00\% & 2.45 \\
%     20 & 700 $\rightarrow$ 500 & 0.2827 & 0.6391 &0.6714 &100.00\%& 9.65 \\

%     \bottomrule
%     \end{tabular}
%     }
% \end{table}
As shown in Tab.~\ref{tab:overall_ablation_analysis_normal}, Tab.~\ref{tab:overall_ablation_analysis_style}, and Tab.~\ref{tab:overall_ablation_analysis_editing} we conduct ablation study of main improvements on different settings. The modules AP (Adaptive Position), DAM (Dynamic Attention Modulation), and PI (Prompt Intensification) effectively maintain consistency in the generated images across all three settings.

\begin{table}[!htbp]
\setlength{\tabcolsep}{4pt}
\caption{Ablation study of the main improvements under the NORMAL setting: adaptive position (AP), dynamic attention modulation (DAM), and prompt intensification (PI) on the CelebA-TV2I validation set.}
\vspace{5mm} % Adjust vertical space above the table
\centering
\setlength{\aboverulesep}{0pt} % No space above the horizontal rules
\setlength{\belowrulesep}{0pt} % No space below the horizontal rules
\scalebox{1}{
\begin{tabular}{ccc|cc}
    \toprule
     AP & DAM & PI & ID-Distance $\downarrow$ & Failure Rate $\downarrow$ \\ \hline \hline
    \xmark & \xmark & \xmark & 0.628 & 20.00\% \\
    \cmark & \xmark & \xmark & 0.643 & 10.00\% \\
    \cmark & \cmark & \xmark & 0.621 & 5.00\% \\
    \cmark & \cmark & \cmark & \textbf{0.604} & \textbf{0.00\%} \\
    \bottomrule
\end{tabular}}
\vspace{-1mm} % Adjust vertical space below the table
\label{tab:overall_ablation_analysis_normal}
\end{table}

\begin{table}[!htbp]
\setlength{\tabcolsep}{4pt}
\caption{Ablation study of the main improvements under the STYLE TRANSFER setting: adaptive position (AP), dynamic attention modulation (DAM), and prompt intensification (PI) on the CelebA-TV2I validation set.}
\vspace{5mm} % Adjust vertical space above the table
\centering
\setlength{\aboverulesep}{0pt} % No space above the horizontal rules
\setlength{\belowrulesep}{0pt} % No space below the horizontal rules
\scalebox{1}{
\begin{tabular}{ccc|cc}
    \toprule
      AP & DAM & PI & ID-Distance $\downarrow$ & Failure Rate $\downarrow$ \\ \hline \hline
    \xmark & \xmark & \xmark & 0.822 & 10.00\% \\
    \cmark & \xmark & \xmark & \textbf{1.098} & 20.00\% \\
    \cmark & \cmark & \xmark & 1.122 & \textbf{10.00\%} \\
    \cmark & \cmark & \cmark & \textbf{1.098} & \textbf{10.00\%}\\
    \bottomrule
\end{tabular}}
\vspace{-1mm} % Adjust vertical space below the table
\label{tab:overall_ablation_analysis_style}
\end{table}

\begin{table}[!htbp]
\setlength{\tabcolsep}{5pt}
\caption{Ablation study of the main improvements under the ATTRIBUTE EDITING setting: adaptive position (AP), dynamic attention modulation (DAM), and prompt intensification (PI) on the CelebA-TV2I validation set.}
\vspace{5mm} % Adjust vertical space above the table
\centering
\setlength{\aboverulesep}{0pt} % No space above the horizontal rules
\setlength{\belowrulesep}{0pt} % No space below the horizontal rules
\scalebox{1}{
\begin{tabular}{ccc|cc}
    \toprule
      AP & DAM & PI & ID-Distance $\downarrow$ & Failure Rate $\downarrow$ \\ \hline \hline
    \xmark & \xmark & \xmark & 0.881 & 20.00\% \\
    \cmark & \xmark & \xmark & 0.730 & 10.00\% \\
    \cmark & \cmark & \xmark & \textbf{0.684} & 10.00\% \\
    \cmark & \cmark & \cmark & 0.718 & \textbf{5.00\%} \\
    \bottomrule
\end{tabular}}
\vspace{-1mm} % Adjust vertical space below the table
\label{tab:overall_ablation_analysis_editing}
\end{table}

\section*{Properties of Diffusion Generation Process} \label{sec:properties}
\begin{figure}[!h]
    \centering
    \includegraphics[width=0.5\textwidth]{images/addtext_clip.pdf}
    \caption{Text-sensitivity during denoising process. Each line represents a CLIP cosine similarity between the generated image and text with the text condition injected at different steps. The image is generated in 1000 overall unconditional denoising process with 100 steps text conditional guidance starting from $t$. Generally, the denoising process is more responsive to the text condition in the beginning and almost stops reacting to the text condition when high-level semantics are settled.}
    \label{text_sensitivity}
\end{figure}
\subsection{Sensitivity to Text Condition during Denoising}\label{sec:text-sensitivity}
We study the sensitivity of diffusion models to text conditions during the denoising process by injecting text conditions at different denoising steps. We replace a few unconditional denoising steps with text-conditioned ones during the generation of the image randomly sampled from Gaussian noise. We calculate the CLIP cosine similarity between the final generated image and text condition. As shown in Fig.~\ref{text_sensitivity}, the model is more sensitive to text conditions in the early denoising stage and less sensitive in the late stage. This also demonstrates our method reasonably utilizes the sensitivity to text conditions through proposed Seed Initialization and Cyclic One-Way Diffusion.

\subsection{Illustration of Semantic Formation Process of Diffusion Generation}\label{sec:diff-size_semantic_formation}

To quantitatively assess the influence between regions during the denoising process, we inverse an image $x_0$ to obtain different transformed $\mathbf{x_t}$, and plant it in a replacement manner into a sub-region of random Gaussian noise in the same step. We subsequently apply this composite noise map to several denoising steps before extracting the planted image to continue the generation process. As shown in Fig.~\ref{fig:measure_influence_along_denoise_process}, the influence level weakens with the denoising process. 

To see the degree of impact exerted on images of different sizes during the denoising process, we conduct the same experiments with images of two different sizes ($128\times128$, $256\times256$). We inverse images to $\mathbf{x_t}$, and reconstruct them with disturbance introduced by sticking them to a random noise background ($512 \times 512$) at the corresponding step for 100 steps. We calculate the MSE loss of the original image and the final reconstructed image after being disturbed. As shown in Fig.~\ref{fig:size-mse}, the semantics settle earlier when the size is larger.

\vspace{-1cm}
\begin{figure}[!h]
    \centering
    \includegraphics[width=0.5\textwidth]{images/size-mse.pdf}
    \caption{Different sizes come with different semantic formation processes. Each red curve represents a face disturb-and-reconstruct process, (a) size is $256 \times 256$ and (b) size is $128 \times 128$. We disturb the reconstruction process by sticking the origin image to a random noise background ($512 \times 512$) at different steps. The general semantic is settled earlier when the size is larger.}
    \label{fig:size-mse}
\end{figure}
\vspace{-10cm}
\begin{figure}[!h]
    \centering
    \includegraphics[width=0.45\textwidth]{images/cos.pdf}
    % \vspace{-3mm}
    \caption{Illustration of the semantic formation process and the mutual interference. Each red curve represents a face disturb-and-reconstruct process. We only show one face for instance. We disturb the reconstruction process by sticking the origin image to a random noise background at different steps. The cosine similarity between the original image and the reconstructed image increases as the denoising step goes. 
    }
    \label{fig:measure_influence_along_denoise_process}
\end{figure}
 \begin{figure*}[!t]
    \centering
    \includegraphics[width=0.7\textwidth]{images/compare_newb3.pdf}
    \caption{Comparison of our SOW-generated images with TV2I baselines.}
    \label{compare}
\end{figure*}

\vfill
